# Supplementary material for: Computation of the heat capacity of water from first principles
Source: arXiv:2509.19765 source file (2025-09-24)
Supplement: Supplementary file 1 [file SI.pdf]

## Supplementary Material : Computation of the heat capacity of water from first principles

Motoyuki Shiga,<sup>1, a)</sup> Jan Elsner,<sup>2, 3</sup> Jörg Behler,<sup>2, 3</sup> and Bo Thomsen<sup>1</sup>

<sup>1)</sup>*Center for Computational Science and e-Systems, Japan Atomic Energy Agency, Kashiwa, Chiba 277-0871, Japan*

<sup>2)</sup>*Lehrstuhl für Theoretische Chemie II, Ruhr-Universität Bochum, 44780 Bochum, Germany*

<sup>3)</sup>*Research Center Chemical Sciences and Sustainability, Research Alliance Ruhr, 44780 Bochum, Germany*

(Dated: 24 September 2025)

This is the supplementary information for the paper "Computation of the heat capacity of water from first principles". Here we present the extended comparison of the radial distribution functions (RDFs) calculated from the simulations carried out in the main article, and the experiments carried out by Soper.<sup>1,2</sup> We also analyze the energy autocorrelation function to evaluate the adequacy of sampling in the MD and PIMD trajectories.

---

<sup>a)</sup>Electronic mail: shiga.motoyuki@jaea.go.jp

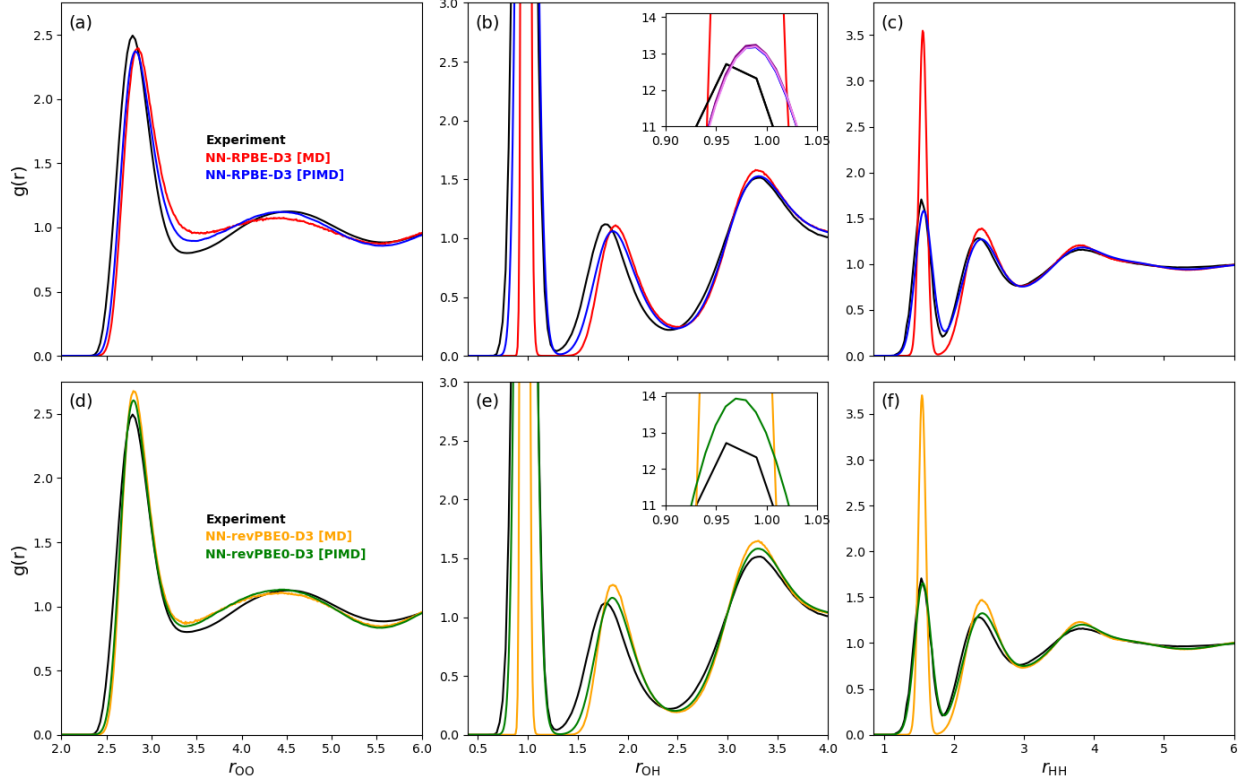

FIG. S1. Comparison of the (a,d) O-O, (b,e) O-H, and (c,f) H-H RDFs of the simulations carried out in this study with experiment. The experimental RDFs (black) are taken from Ref. 2 for the O-O RDFs and from Ref. 1 for the O-H and H-H RDFs. The inserts in (b,e) are added to compare the position of the first O-H RDF peak for the PIMD simulations with the experimental peak, all MD results display a much sharper first O-H peak with a  $g(r_{\max}) \approx 40 - 45$ . In (a-c) we compare the RDFs of the NN-RPBE-D3 potential using MD (red) with those obtained from PIMD (blue) simulations. In (d-f) we compare the RDFs of the NN-revPBE0-D3 potential using MD (orange) with those obtained from PIMD (green).

## REFERENCES

- <sup>1</sup>A. K. Soper, Chem. Phys. **258**, 121 (2000).
- <sup>2</sup>A. K. Soper, ISRN Physical Chemistry **2013**, e279463 (2013).

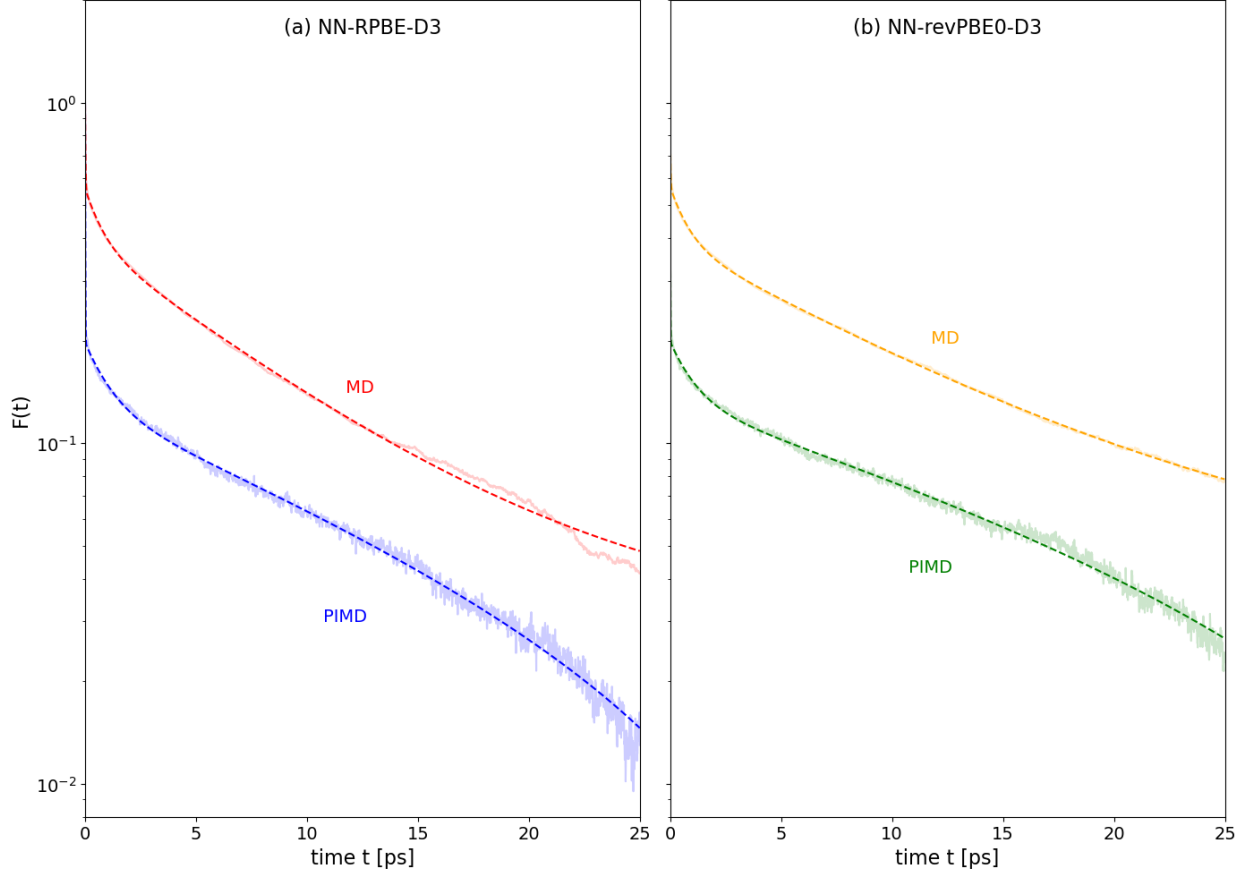

FIG. S2. The normalized energy autocorrelation function from the MD and PIMD trajectories, which is defined as  $F(t) = \frac{\langle (\epsilon_{\text{CV}}(t) - \langle \epsilon_{\text{CV}} \rangle) (\epsilon_{\text{CV}}(0) - \langle \epsilon_{\text{CV}} \rangle) \rangle}{\langle (\epsilon_{\text{CV}}(0) - \langle \epsilon_{\text{CV}} \rangle) (\epsilon_{\text{CV}}(0) - \langle \epsilon_{\text{CV}} \rangle) \rangle}$ . The results are shown for (a) MD (red) and PIMD trajectories using the NN-RPBE-D3 potential, and (b) MD (orange) and PIMD (green) trajectories using the NN-revPBE0-D3 potential. In all cases, the shaded regions represent raw data from the trajectories, while dashed lines indicate the fits to a sum of three exponential functions. The fitting parameters are listed in Table SI. Note that this analysis is performed solely to verify that the energy sampling is sufficient. It does not provide the real-time information, as the MD and PIMD trajectories are strongly thermostatted to ensure efficient sampling.

TABLE SI. The fitting parameters for the normalized energy autocorrelation function in Figure S2 to the expression  $F(t) = A_0 + A_1 \exp(t/\tau_1) + A_2 \exp(t/\tau_2) + A_3 \exp(t/\tau_3)$ . The  $\tau_i$  has been sorted according to timescales, so that  $\tau_1 \approx 7 - 16$  fs,  $\tau_2 \approx 0.7 - 1.2$  ps and  $\tau_3 \approx 8 - 25$  ps, respectively.

|                      | $A_0$                 | $A_1$ | $\tau_1$ [ps]        | $A_2$                | $\tau_2$ [ps] | $A_3$ | $\tau_3$ [ps] |
|----------------------|-----------------------|-------|----------------------|----------------------|---------------|-------|---------------|
| NN-RPBE-D3 (MD)      | $-2.20 \cdot 10^{-2}$ | 0.801 | $7.81 \cdot 10^{-3}$ | $7.00 \cdot 10^{-2}$ | 1.15          | 0.149 | 17.8          |
| NN-RPBE-D3 (PIMD)    | $2.93 \cdot 10^{-2}$  | 0.429 | $1.55 \cdot 10^{-2}$ | $1.68 \cdot 10^{-1}$ | 0.788         | 0.362 | 8.47          |
| NN-revPBE0-D3 (MD)   | $-3.27 \cdot 10^{-2}$ | 0.800 | $7.66 \cdot 10^{-3}$ | $6.66 \cdot 10^{-2}$ | 1.10          | 0.165 | 24.5          |
| NN-revPBE0-D3 (PIMD) | $4.08 \cdot 10^{-2}$  | 0.422 | $1.47 \cdot 10^{-2}$ | $1.77 \cdot 10^{-1}$ | 0.811         | 0.349 | 11.2          |
